# Supplementary material for: Remote Identification Trajectory Coverage in Urban Air Mobility Applications
Source: arXiv:2302.09653 source file (2023-02-19)
Supplement: Supplementary file 2 [file 7_appendix.tex]

\section{Appendix}  \label{sec:appendix}

This is tables.
\begin{table}[ht]
  \centering
  \caption{Number of Receivers Needed to Achieve Coverage $\%$ for OD Paths}
    \begin{tabular}{p{0.018\textwidth}<{\centering}p{0.018\textwidth}<{\centering}p{0.018\textwidth}<{\centering}p{0.018\textwidth}<{\centering}p{0.018\textwidth}<{\centering}p{0.018\textwidth}<{\centering}p{0.018\textwidth}<{\centering}p{0.018\textwidth}<{\centering}p{0.018\textwidth}<{\centering}p{0.018\textwidth}<{\centering}p{0.0175\textwidth}<{\centering}}
    \hline
    \multirow{2}{*}{\textbf{City}} 
     & \multicolumn{3}{c}{\textbf{R250}} &\multicolumn{3}{c}{\textbf{R1000}}&\multicolumn{3}{c}{\textbf{R2000}} &  \multirow{1}{*}{\textbf{Alt.}} \\ 
     & $50\%$     & $75\%$     & $95\%$     &  $50\%$     & $75\%$     & $95\%$  &  $50\%$     & $75\%$     & $95\%$   & (ft.)\\\hline
     \multirow{2}{*}{\textbf{SF}} & 2 &3&4&5&6&7&8&9&10&200\\
     & 2 &3&4&5&6&7&8&9&10&400\\
    \hline
     \multirow{2}{*}{\textbf{NYC}}& 2 &3&4&5&6&7&8&9&10&200\\
     & 2 &3&4&5&6&7&8&9&10&400\\
    \hline
     \multirow{2}{*}{\textbf{LA}}& 2 &3&4&5&6&7&8&9&10&200\\
     & 2 &3&4&5&6&7&8&9&10&400\\
    \hline
    \end{tabular}%
  \label{tab:1_sheet3}%
\end{table}

\begin{table}[ht]
  \centering
  \caption{Number of Receivers Needed to Achieve Coverage $\%$ for RRT* Paths}
     \begin{tabular}{p{0.018\textwidth}<{\centering}p{0.018\textwidth}<{\centering}p{0.018\textwidth}<{\centering}p{0.018\textwidth}<{\centering}p{0.018\textwidth}<{\centering}p{0.018\textwidth}<{\centering}p{0.018\textwidth}<{\centering}p{0.018\textwidth}<{\centering}p{0.018\textwidth}<{\centering}p{0.018\textwidth}<{\centering}p{0.0175\textwidth}<{\centering}}
    \hline
    \multirow{2}{*}{\textbf{City}} 
     & \multicolumn{3}{c}{\textbf{R250}} &\multicolumn{3}{c}{\textbf{R1000}}&\multicolumn{3}{c}{\textbf{R2000}} &  \multirow{1}{*}{\textbf{Alt.} } \\ 
     & \textbf{$50\%$}     & \textbf{$75\%$}     & \textbf{$95\%$}     & \textbf{$50\%$}     & \textbf{$75\%$}     & \textbf{$95\%$} & \textbf{$50\%$}     & \textbf{$75\%$}     & \textbf{$95\%$}  & (ft.)\\\hline
     \multirow{2}{*}{\textbf{SF}} & 2 &3&4&5&6&7&8&9&10&200\\
     & 2 &3&4&5&6&7&8&9&10&400\\
    \hline
     \multirow{2}{*}{\textbf{NYC}}& 2 &3&4&5&6&7&8&9&10&200\\
     & 2 &3&4&5&6&7&8&9&10&400\\
    \hline
     \multirow{2}{*}{\textbf{LA}}& 2 &3&4&5&6&7&8&9&10&200\\
     & 2 &3&4&5&6&7&8&9&10&400\\
    \hline
    \end{tabular}%
  \label{tab:2_sheet3}%
\end{table}



% \begin{table}[ht]
%   \centering
%   \caption{Number of Receivers Needed to Achieve Coverage $\%$for VG Paths}
%   \begin{tabular}{p{0.018\textwidth}<{\centering}p{0.018\textwidth}<{\centering}p{0.018\textwidth}<{\centering}p{0.018\textwidth}<{\centering}p{0.018\textwidth}<{\centering}p{0.018\textwidth}<{\centering}p{0.018\textwidth}<{\centering}p{0.018\textwidth}<{\centering}p{0.018\textwidth}<{\centering}p{0.018\textwidth}<{\centering}p{0.0175\textwidth}<{\centering}}
%     \hline
%     \multirow{2}{*}{\textbf{City}} 
%      & \multicolumn{3}{c}{\textbf{R250}} &\multicolumn{3}{c}{\textbf{R1000}}&\multicolumn{3}{c}{\textbf{R2000}} &  \multirow{1}{*}{\textbf{Alt.}} \\ 
%      & \textbf{$50\%$}     & \textbf{$75\%$}     & \textbf{$95\%$}     & \textbf{$50\%$}     & \textbf{$75\%$}     & \textbf{$95\%$} & \textbf{$50\%$}     & \textbf{$75\%$}     & \textbf{$95\%$} & (ft.) \\\hline
%      \multirow{2}{*}{\textbf{SF}} & 2 &3&4&5&6&7&8&9&10&200\\
%      & 2 &3&4&5&6&7&8&9&10&400\\
%     \hline
%      \multirow{2}{*}{\textbf{NYC}}& 2 &3&4&5&6&7&8&9&10&200\\
%      & 2 &3&4&5&6&7&8&9&10&400\\
%     \hline
%      \multirow{2}{*}{\textbf{LA}}& 2 &3&4&5&6&7&8&9&10&200\\
%      & 2 &3&4&5&6&7&8&9&10&400\\
%     \hline
%     \end{tabular}%
%   \label{tab:3_sheet3}%
% \end{table}



% \begin{table}[ht]
%   \centering
%   \caption{Performance Comparison on the PE and RT}
%     \begin{tabular}{p{0.023\textwidth}<{\centering}p{0.06\textwidth}<{\centering}p{0.06\textwidth}<{\centering}p{0.06\textwidth}<{\centering}p{0.06\textwidth}<{\centering}p{0.05\textwidth}<{\centering}}
%     \hline
%     \multirow{2}{*}{\textbf{City}} & \multicolumn{2}{c}{\textbf{RRT$^*$}}     &  \multicolumn{2}{c}{\textbf{VG}} &  \multirow{1}{*}{\textbf{Alt.}}   \\
%     &PE &RT&PE &RT& (ft.)\\
%     \hline
%  \multirow{2}{*}{\textbf{SF}} & 2 &3&4&5&200\\
%      & 2 &3&4&5&400\\
%     \hline
%      \multirow{2}{*}{\textbf{NYC}} & 2 &3&4&5&200\\
%      & 2 &3&4&5&400\\
%      \hline
%      \multirow{2}{*}{\textbf{LA}} & 2 &3&4&5&200\\
%      & 2 &3&4&5&400\\
%     \hline
%      \multicolumn{6}{c}{PE: Path Efficiency\;\; RT: Run Time}\\
%      \hline
%     \end{tabular}%
%   \label{tab:1_sheet4}%
% \end{table}


\begin{table}[ht]
  \centering
  \caption{Breakdown of Receiver Technologies Based on Range}
    \begin{tabular}{ccc}
    \hline
    \multirow{1}{*}{Case Study Group} & \multicolumn{1}{c}{Radius}     &  \multicolumn{1}{c}{Technology} \\
    \hline
 \multirow{1}{*}{\textbf{R250}} & 250m &Bluetooth Legacy Advertising\\
 \multirow{1}{*}{\textbf{R1000}} & 1km &Bluetooth Long Range\\
\multirow{1}{*}{\textbf{R2000}} & 2km &Wi-Fi NAN, Wi-Fi Beacon\\
\multirow{1}{*}{\textbf{R---}} & -- &LoRa\\
    \hline
     % \multicolumn{6}{c}{PE: Path Efficiency\;\; RT: Run Time}\\
     % \hline
    \end{tabular}%
  \label{tab:1_sheet1}%
\end{table}


\begin{table*}
  \centering
  \caption{Environment Comparison}
    \begin{tabular}{cccccc}
    \hline
    \multirow{1}{*}{\textbf{City}} & \multicolumn{1}{c}{*Pop. Per Sqr Mile}     &  \multicolumn{1}{c}{**Stores Per Sqr Kilometer} &  \multirow{1}{*}{**Bldg. Per Sqr Mile} &  \multirow{1}{*}{**Mean Bldg. H.t.} &  \multirow{1}{*}{**Std Bldg. H.t.}   \\
    \hline
 \multirow{1}{*}{\textbf{SF}} & 7193 &3&3723&5&200\\
    % \hline
 \multirow{1}{*}{\textbf{NYC}} & 11314 &3&4739&5&200\\
     % \hline
 \multirow{1}{*}{\textbf{LA}} & 3206 &1&4968&5&200\\
    \hline
     \multicolumn{6}{c}{*\hyperlink{https://www.census.gov/quickfacts/fact/table/losangelescitycalifornia,newyorkcitynewyork,NY,sanfranciscocitycalifornia,sanfranciscocountycalifornia/POP060220}{US Census}\;\; **OSM Dataset Stats}\\
     \hline
    \end{tabular}%
  \label{tab:1_sheet2}%
\end{table*}






% \begin{table*}[ht]
%   \centering
%   \caption{Number of Remote ID receivers needed to achieve coverage proportions (\%) for \textsc{Slpp}, 20 trials of 1,000 trajectories each}
%     \begin{tabular}{p{0.06\textwidth}<{\centering}p{0.06\textwidth}<{\centering}p{0.06\textwidth}<{\centering}p{0.06\textwidth}<{\centering}p{0.06\textwidth}<{\centering}p{0.06\textwidth}<{\centering}p{0.06\textwidth}<{\centering}}
%     % \begin{tabular}{ccccccc}
%     \hline
%     \multirow{2}{*}{} 
%       & \multicolumn{3}{c}{\textbf{Number of Remote ID Receivers}} 
      
%       & \multicolumn{3}{c}{\textbf{Convergence Values (\%)}} \\ 
%       &  $50\%$ & $70\%$ & $95\%$ &  $50\%$  & $70\%$ & $95\%$  \\\hline
%      \multirow{1}{*}{\textbf{R250}} & 525 & 1300 & 5000 & 51.5 & 76.5 & 94.3\\
%     \hline
%      \multirow{1}{*}{\textbf{R1000}} & 30 & 65 & 160 & 51.6 & 74.8 & 94.7\\
%     \hline
%      \multirow{1}{*}{\textbf{R2000}}& 8 & 15 & 35 & 53.7 & 75.5 & 93.4 \\
%     \hline
%     \end{tabular}%
%   \label{tab:1_sheet3}%
% \end{table*}
